# Supplementary material for: Probabilistic Modeling of Semantic Ambiguity for Scene Graph Generation
Source: arXiv:2103.05271 source file (2021-03-10)
Supplement: Supplementary file 1 [file appendix.tex]

\section{Examples of Generated Scene Graph}

\begin{figure*}[ht]
    \centering\includegraphics[width=\textwidth, keepaspectratio]{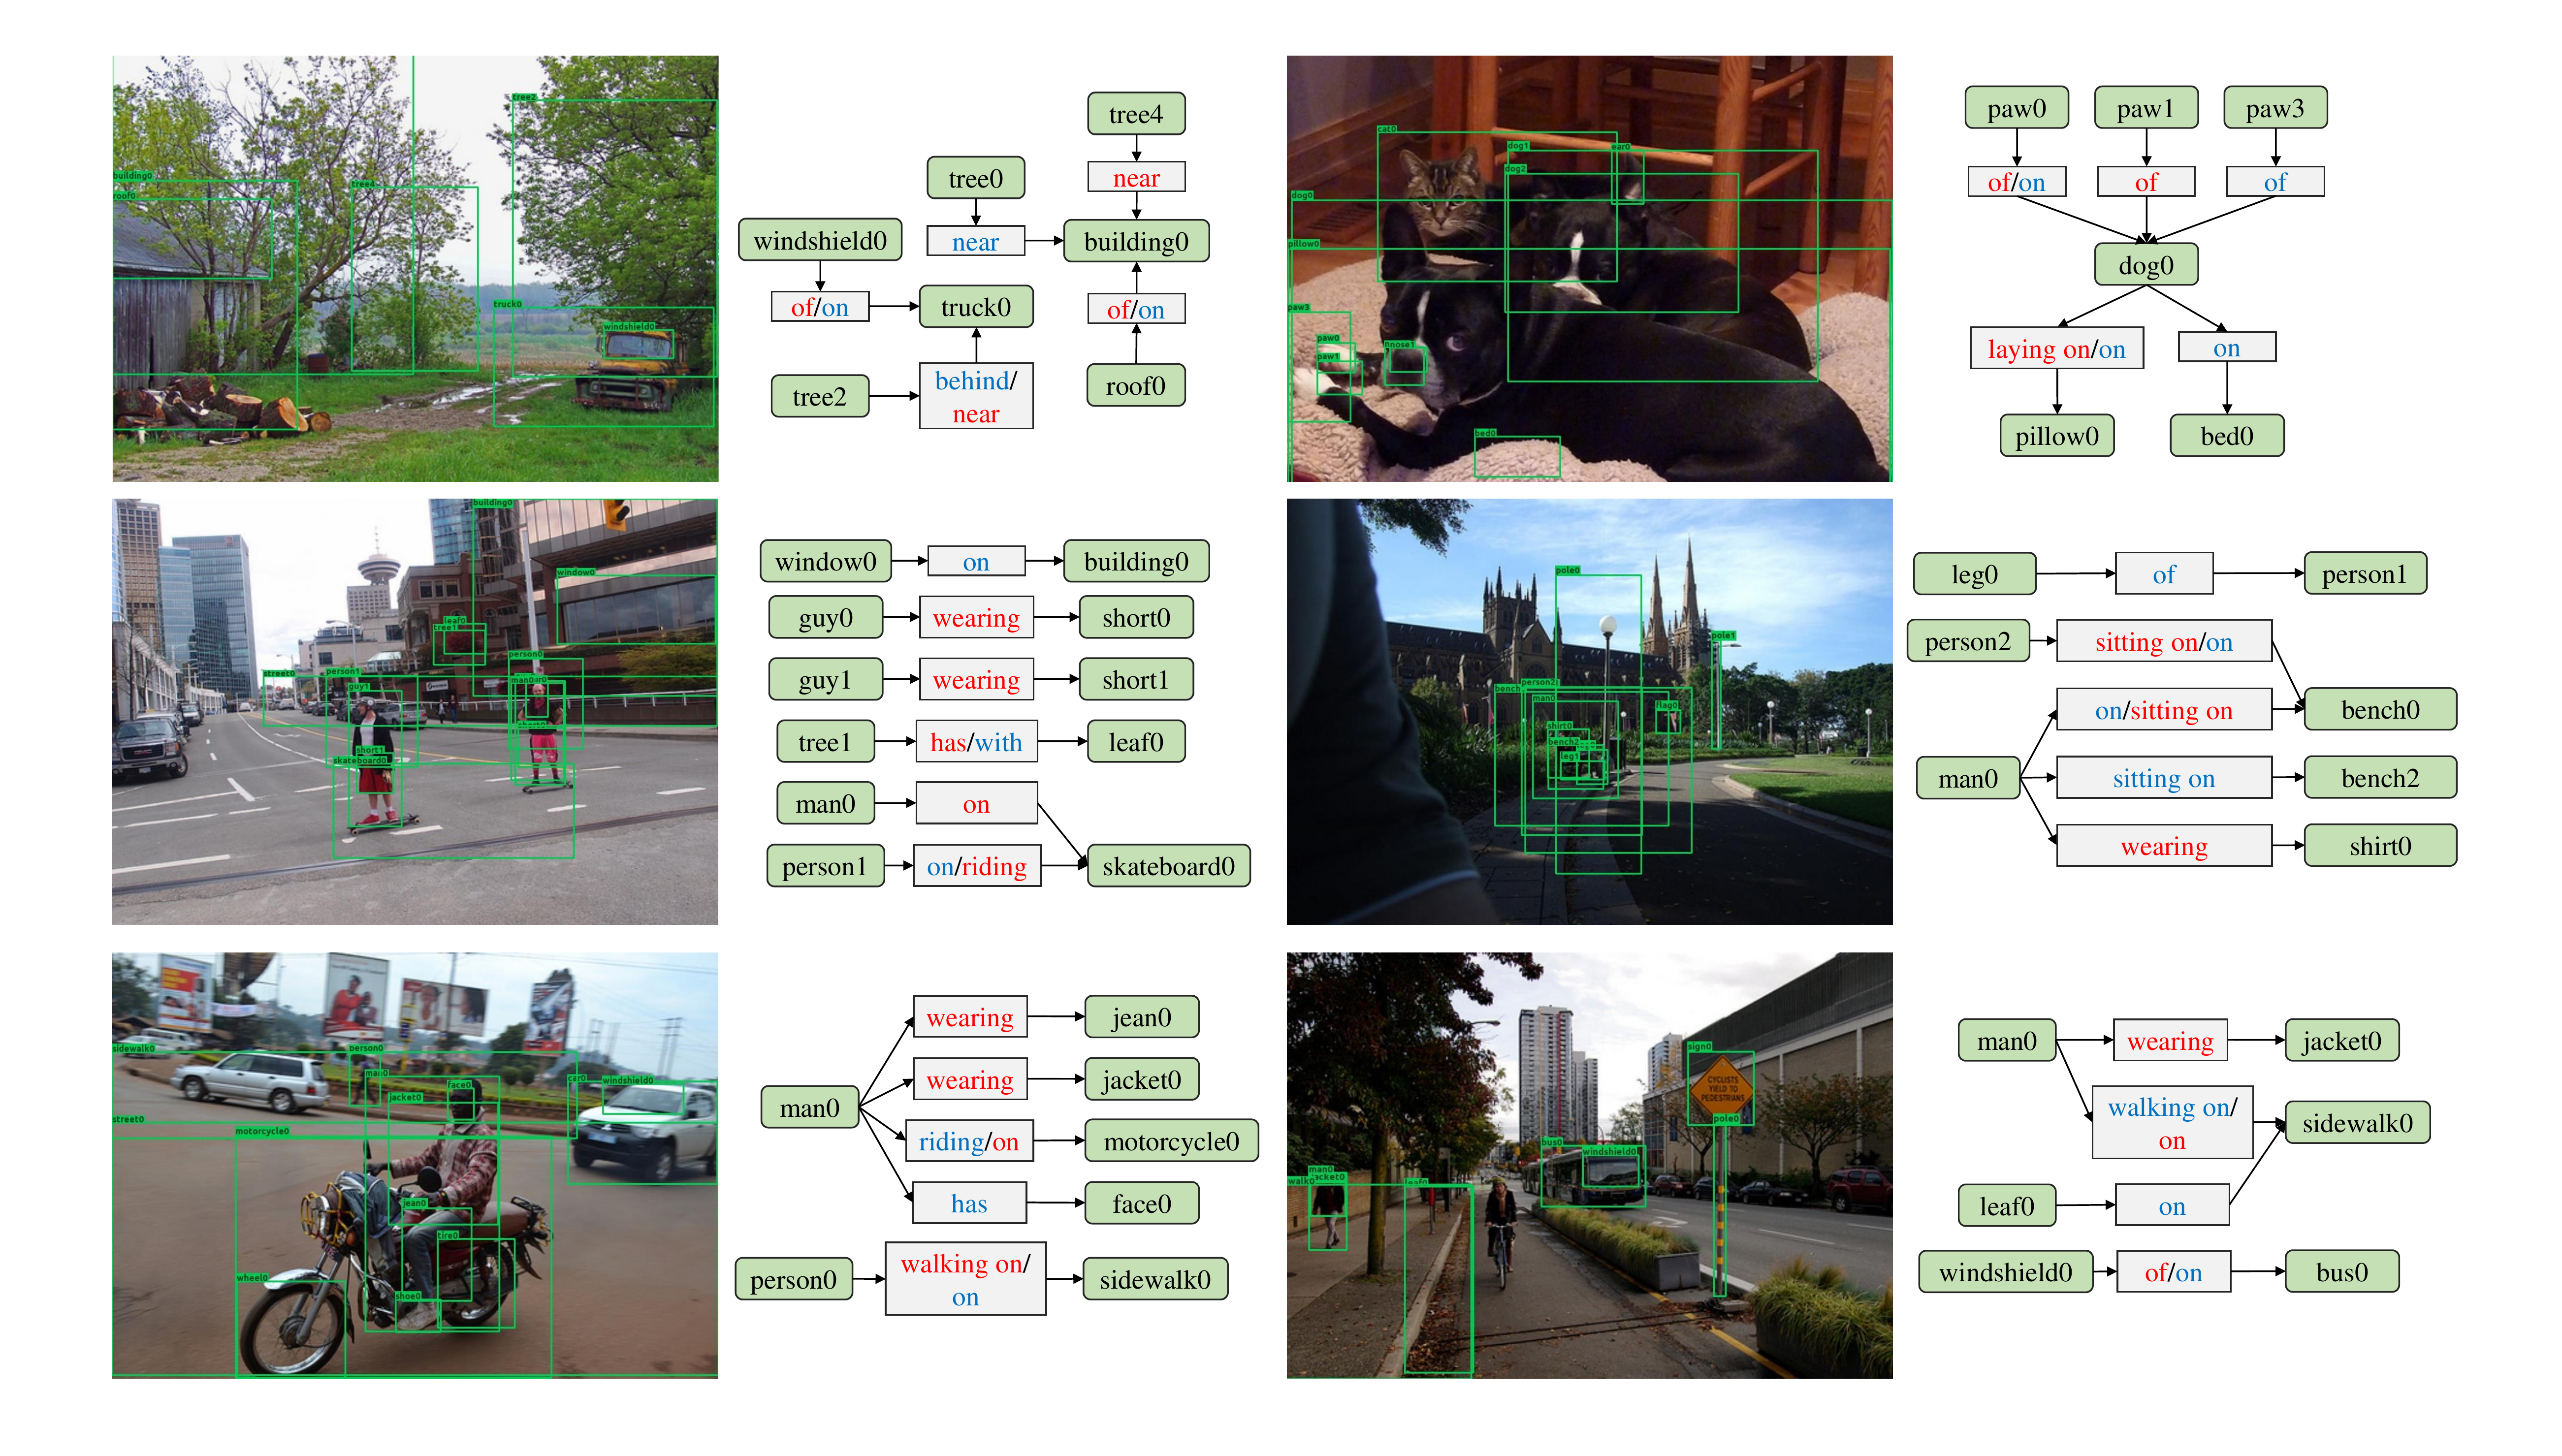}
	\caption{Examples of generated scene graph by ensembling two consecutive inferences in the PredCls setting.
	Blue indicates correctly classified predicates compared to the ground truth;
	red indicates the misclassified ones.}
	\label{fig:scene_graphs}
\end{figure*}

\section{More Ablation Studies}

\begin{table*}
\small
\setlength\tabcolsep{9pt}

\caption{Comparisons of the R@100 and mR@100 in \% of our full model, our model without the conventional deterministic loss in Eq. \ref{eq:ce_loss} (w/o dl), and our model without the regularization term of Eq. \ref{eq:reg_term} (w/o rt).}
\begin{center}
\begin{tabular}{l|c|c|c|c|c|c|c}
\hline
& \multicolumn{2}{c|}{SGDet}
& \multicolumn{2}{c|}{SGCls}
& \multicolumn{2}{c|}{PredCls}
& \\
\hline\hline
Methods &
R@100 & mR@100 &
R@100 & mR@100 &
R@100 & mR@100 \\
\hline
Ours w/o dl & 31.0 & 8.0 & 38.5 & 11.4 & 68.0 & 19.9 \\
Ours w/o rt & 31.2 & 8.3 & 38.5 & 12.2 & 68.3 & 21.6 \\
\textbf{Ours} & \textbf{31.3} & \textbf{8.9} & \textbf{39.0} & \textbf{12.8} & \textbf{68.3} & \textbf{22.0} \\
\hline
\end{tabular}
\end{center}
\label{table:more_ablations}
\end{table*}
